# Supplementary material for: Integrating Deep Learning in Domain Sciences at Exascale
Source: arXiv:2011.11188 source file (2020-11-23)
Supplement: Supplementary file 1 [file appendixA.tex]

\section{Appendix A}
Let matrices $A_{32}$, $B_{32}$ and $C_{32}$ are $N \times N$ matrices in FP32 and assume these
are well approximated by
\begin{align}
A_{32}  & \approx a1_{32} * A1_{16} + a2_{32} * A2_{16} \\
B_{32}  & \approx b1_{32} * B1_{16} + b2_{32} * B2_{16} 
\label{eqn:A_1}
\end{align}
then $C_{32} = A_{32} * B_{32}$ can be approximately computed as
\begin{align}
C_{32}   \approx ~ & (a1_{32} * b1_{32}) * (A1_{16} * B1_{16}) + \\
                 & (a1_{32} * b2_{32}) * (A1_{16} * B2_{16}) + \\
                 & (a2_{32} * b1_{32}) * (A2_{16} * B1_{16}) + \\
                 & (a2_{32} * b2_{32}) * (A2_{16} * B2_{16})
                 ~.
 \label{eqn:A_2}
\end{align}
If we assume 
$a2_{16} = 2^{-11} * a1_{16}$, 
$b2_{16} = 2^{-11} * b1_{16}$, 
then the last contribution is scaled by 
$(a2_{32} * b2_{32}) = 2^{-22} * (a1_{32} * b1_{32})$
which may be optionally dropped without significant errors.
If so, then $C_{32}$ can be computed as 3 matrix multiplies in FP16.
